# Supplementary material for: A modified nudged elastic band algorithm with adaptive spring lengths
Source: arXiv:2106.06275 ancillary file (2021-08-13)
Supplement: Supplementary file 1 [file Supplementary_26July.pdf]

# Supplemental Material: A modified nudged elastic band algorithm with adaptive spring lengths

## 1. Isomerization of alanine dipeptide

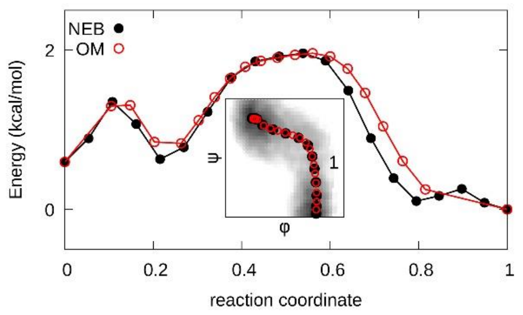


**Figure S1:** Path 1.

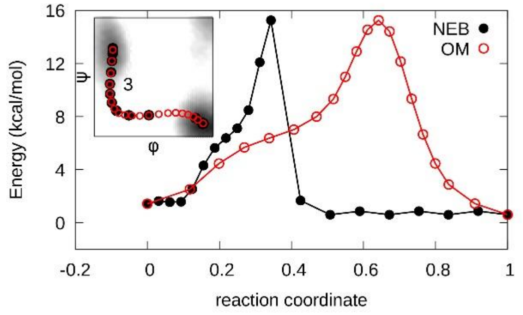


**Figure S2:** Path 3.

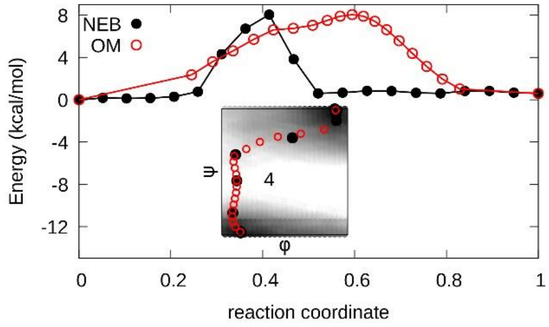


**Figure S3:** Path 4.

**Figure S1-S3:** The potential energy along paths number 1, 3 and 4 (see Figure 1(c) of the main text), obtained using $N = 20$ images. The insets are zoom-in of the paths in the $(\varphi, \psi)$ plane, plotted over the free energy surface. The black and the red curves correspond to the results obtained using the standard and the modified NEB, respectively. The results reported here were obtained using $k_{\parallel} = 1$ kcal/mol/Å$^2$, $k_{\perp} = 0$ and $\nu$ =1 fs$^{-1}$.

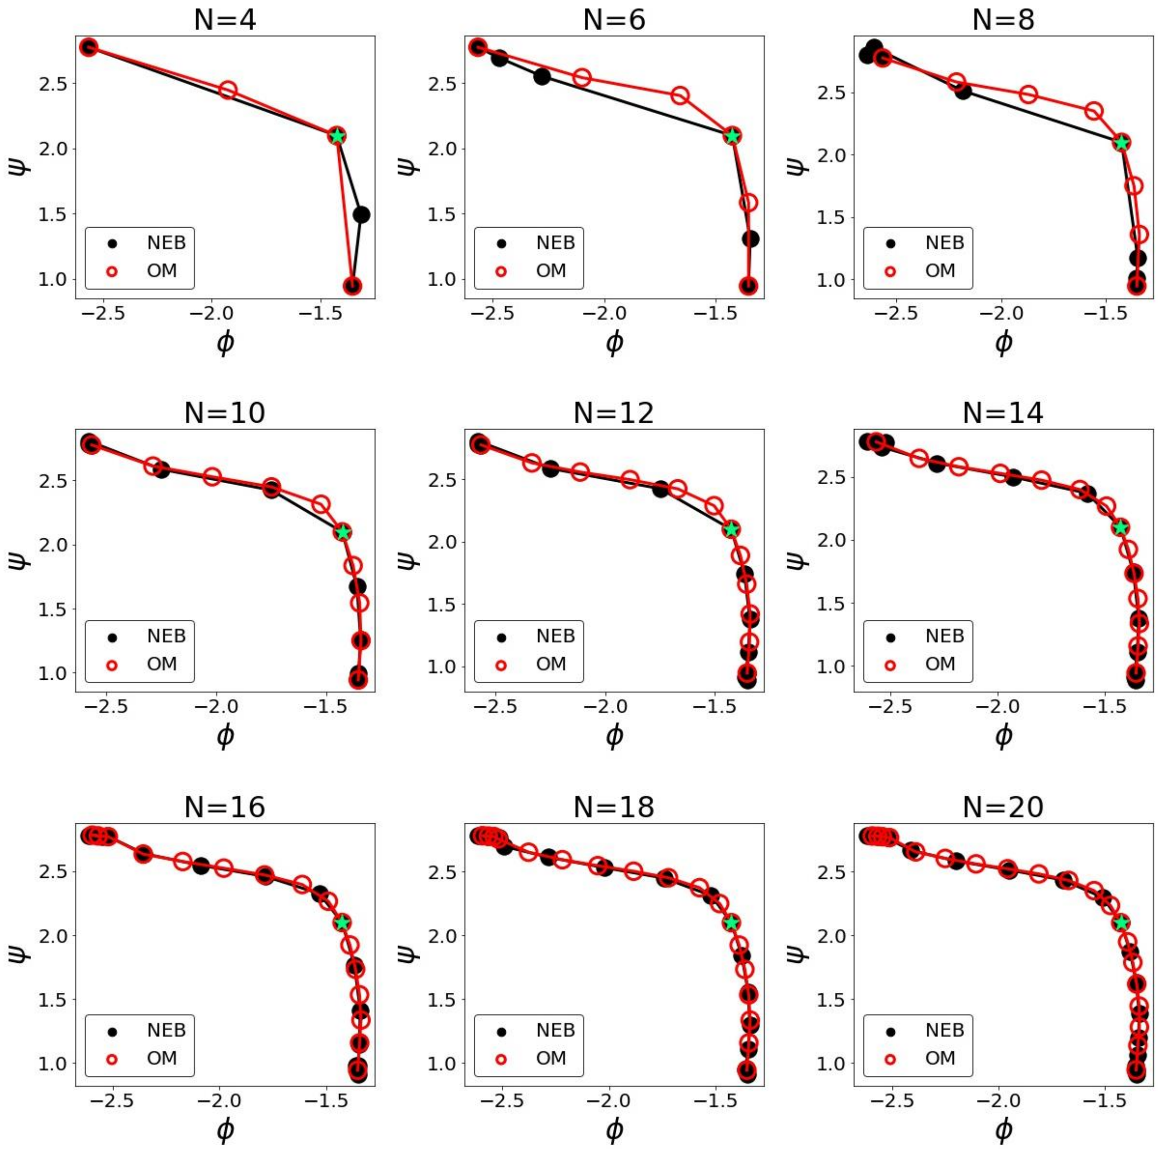


**Figure S4.** Path 1.

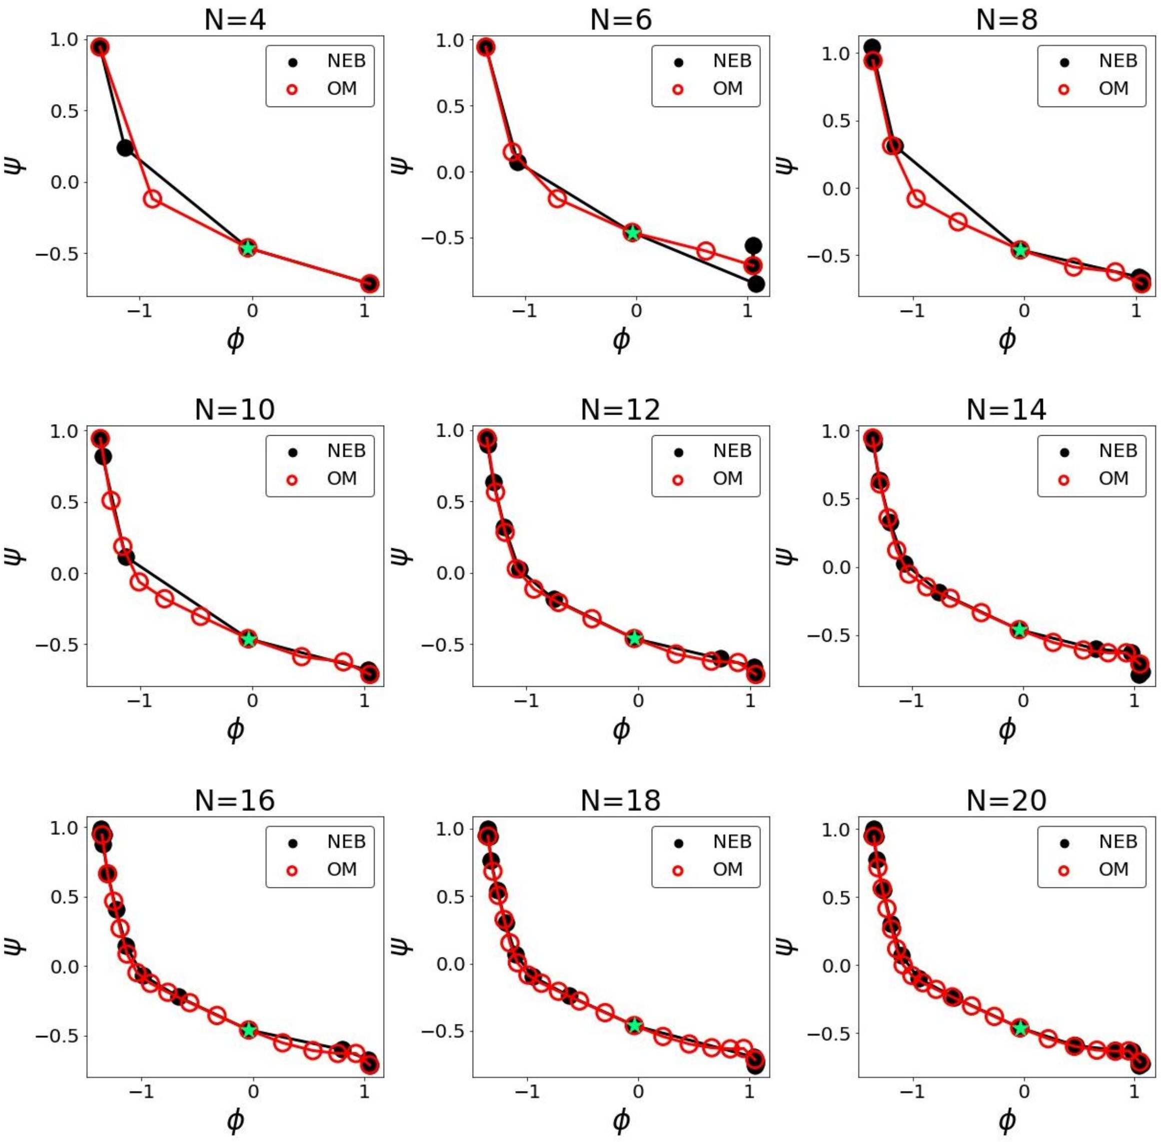


**Figure S5.** Path 2.

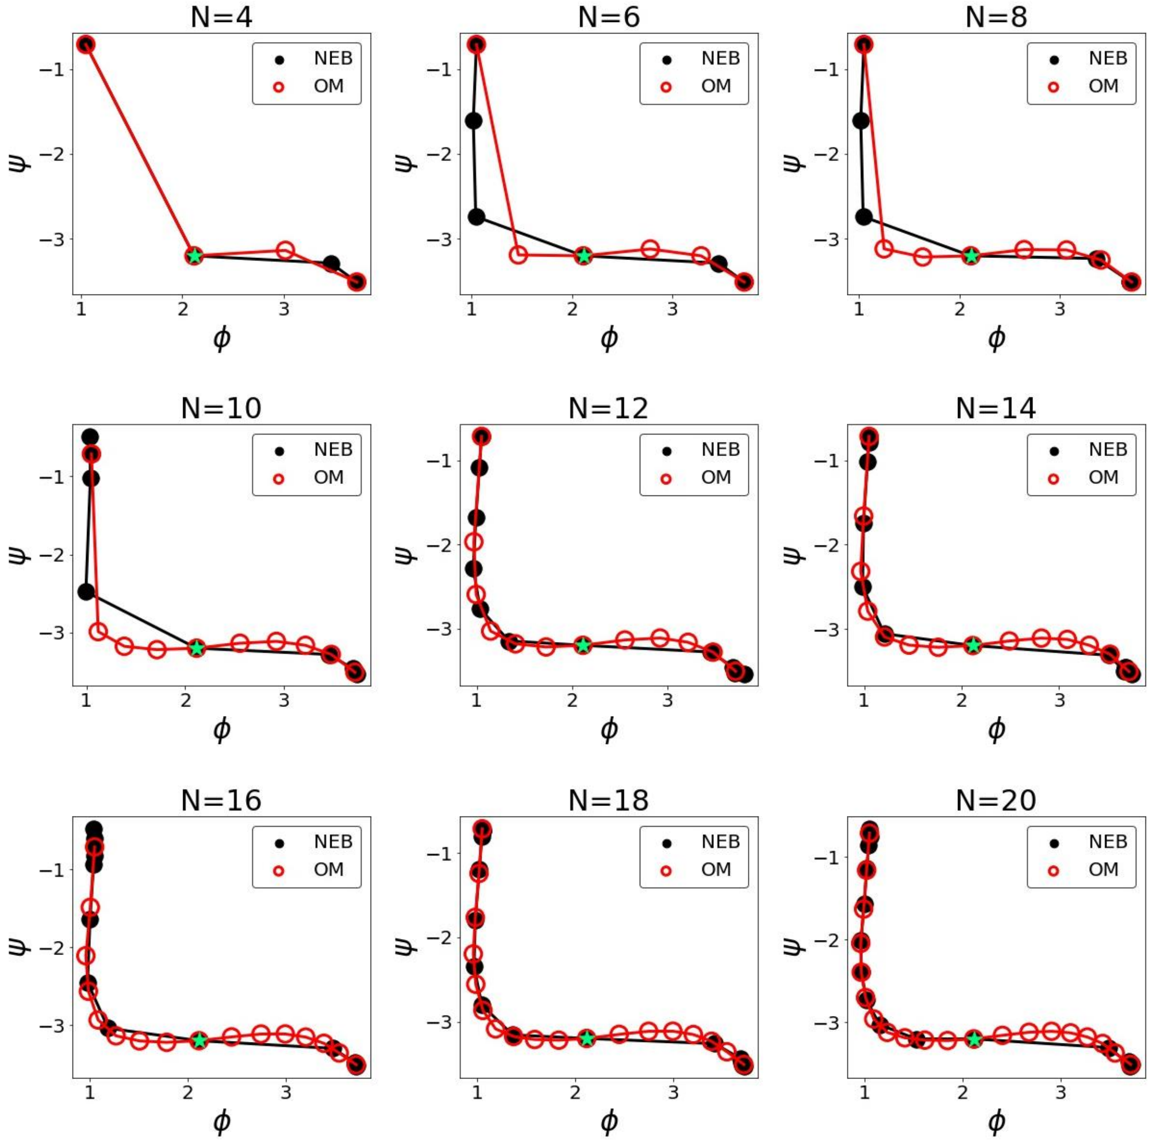


**Figure S6.** Path 3.

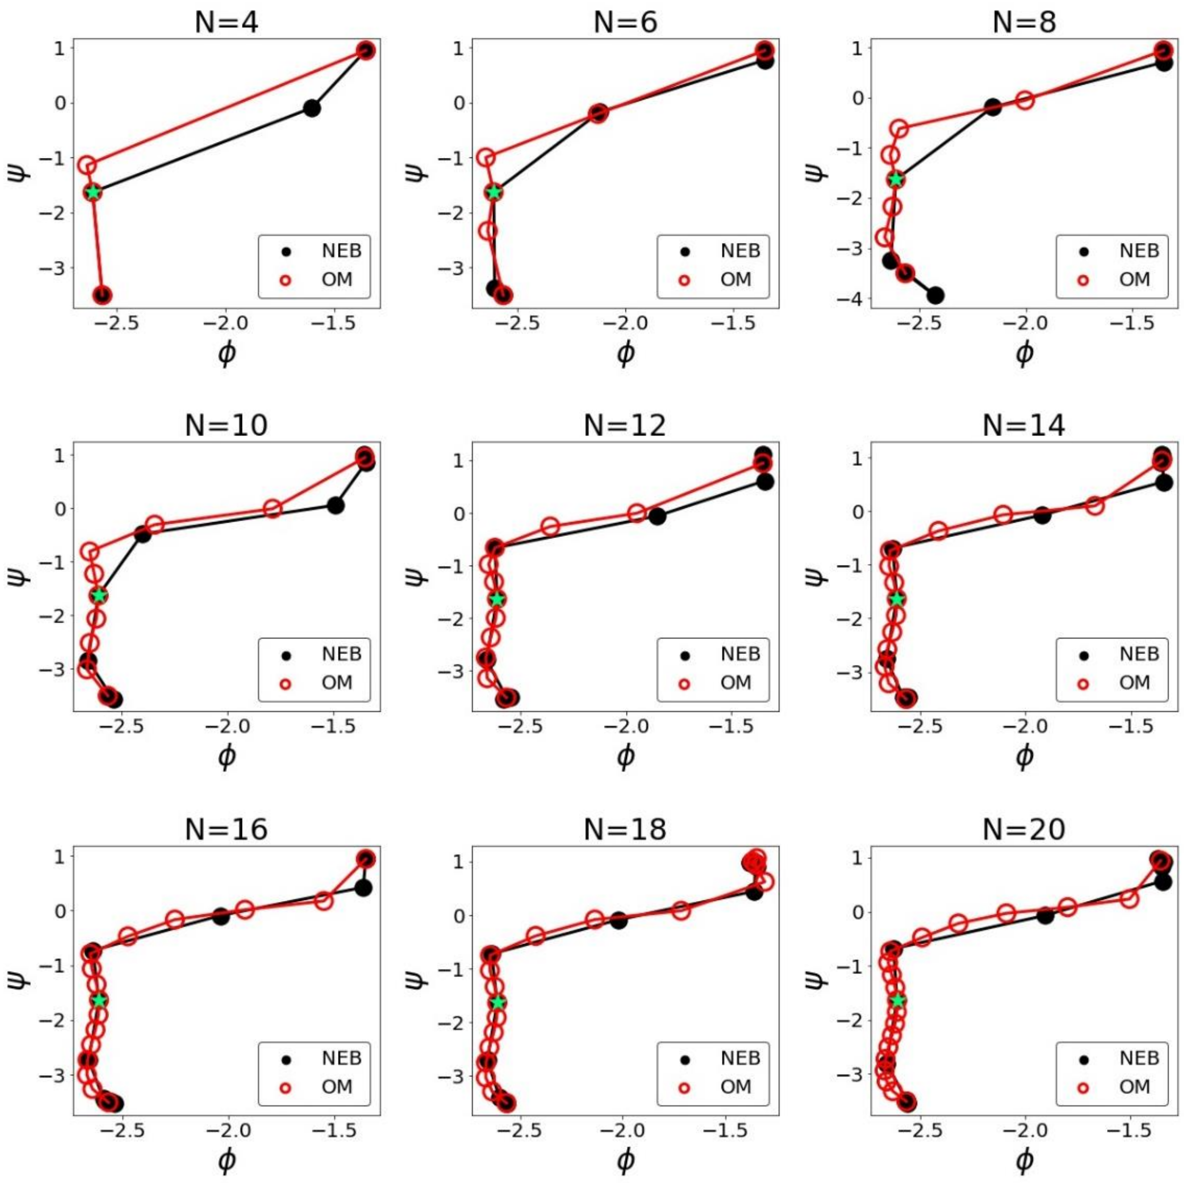


**Figure S7.** Path 4.

**Figure S4-S7:** The MEPs plotted in the $(\varphi, \psi)$ plane corresponding to paths number 1, 2, 3 and 4 (see Figure 1(c) of the main text), respectively. In each figure, different panels are results obtained using an increasing number $N$ of images, as indicated in the title of each panel. The black and the red curves correspond to the results obtained using the standard and the modified NEB, respectively. The results reported here were obtained using $k_{\parallel} = 1$ kcal/mol/Å$^2$, $k_{\perp} = 0$ and $\nu$ =1 fs$^{-1}$. In each panel, the green star marks the image corresponding to the saddle point along the MEP. Both algorithms converge to the exact saddle point, independent of the number of images.

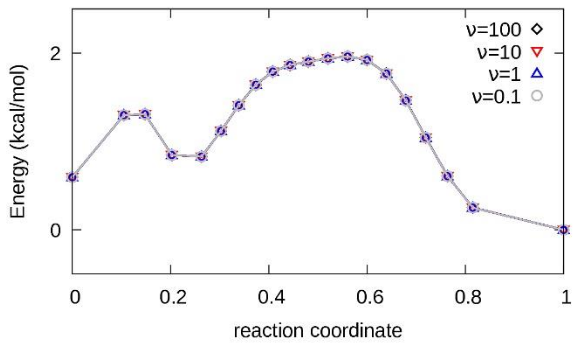


**Figure S8:** Path 1.

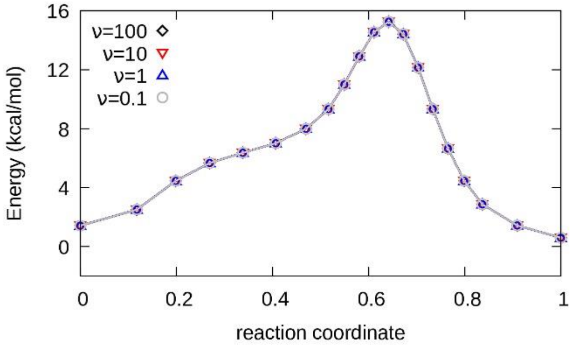


**Figure S9:** Path 3.

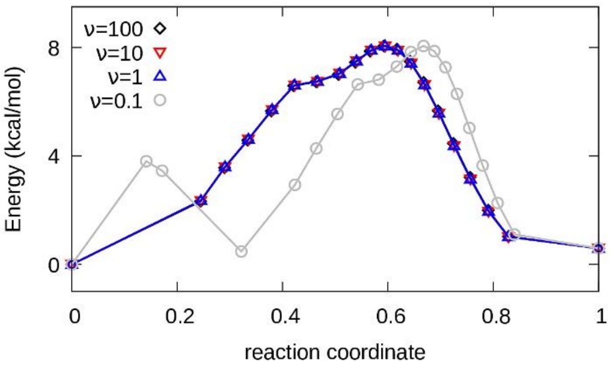


**Figure S10:** Path 4.

**Figure S8-S10:** The potential energy along paths number 1, 3 and 4, obtained using $N = 20$ images and the modified NEB for different values of the parameter $\nu$, defining the mass-dependent spring constant $k_{\mathrm{OM}} = \frac{m\nu}{2\Delta t}$. Values of $\nu$ are indicated in the legend in units of fs$^{-1}$. In all cases, the saddle point identified is independent of the value of $\nu$.

## 2. Elimination of hydrogen from ethane

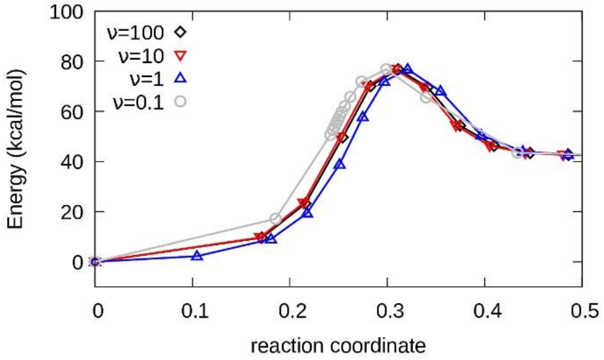


**Figure S11:** The potential energy along the MEP obtained using the modified NEB. Different curves correspond to different values of the parameter $\nu$, as indicated in the legend (units are fs$^{-1}$). The saddle point identified is independent of the value of $\nu$. The results were obtained using $N = 20$ images and only the region around the saddle point is shown. In these simulations, the final configuration of the path corresponds to the hydrogen molecule with its bond parallel to the carbon-carbon bond of ethylene at a distance of 4 Å away from it.

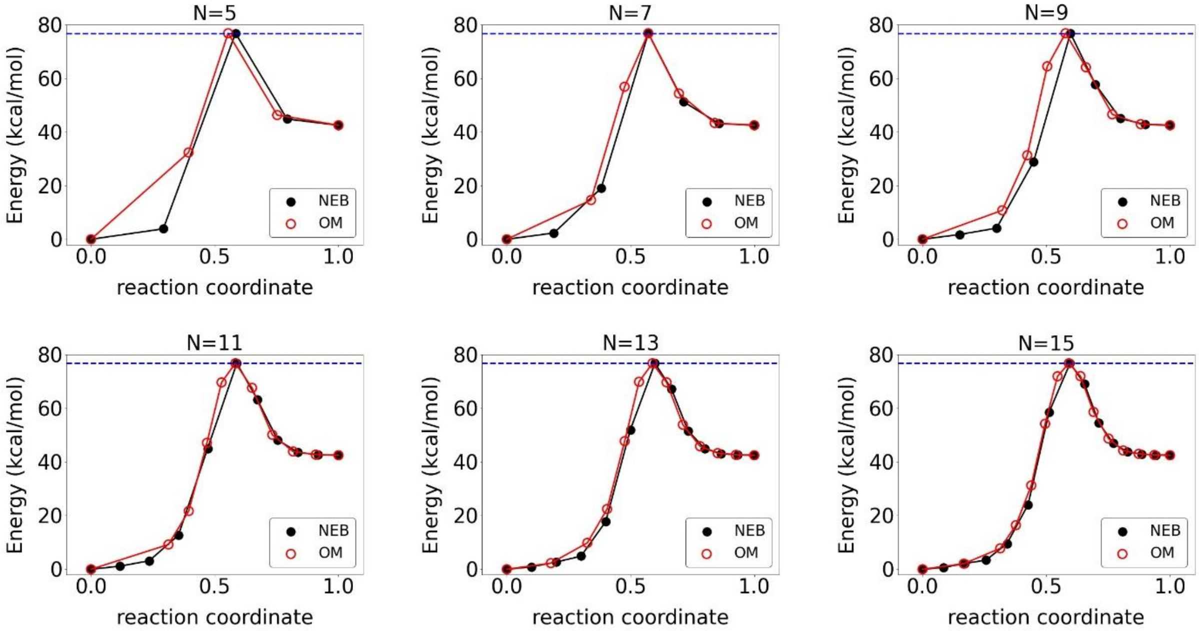


**Figure S12:** The potential energy along the MEPs obtained using an increasing number $N$ of images, as indicated in the title of each panel. The black and the red curves correspond to the results obtained using the standard and the modified NEB, respectively. The results reported here were obtained using $k_{\parallel} = 1$ kcal/mol/Å$^2$, $k_{\perp} = 0$ and $\nu = 1$ fs$^{-1}$. In each panel, the blue dashed line indicates the saddle point energy along the MEP. Both algorithms converge to the exact saddle point, independent of the number of images.

## 3. Healing of a 5-77-5 defect in graphene

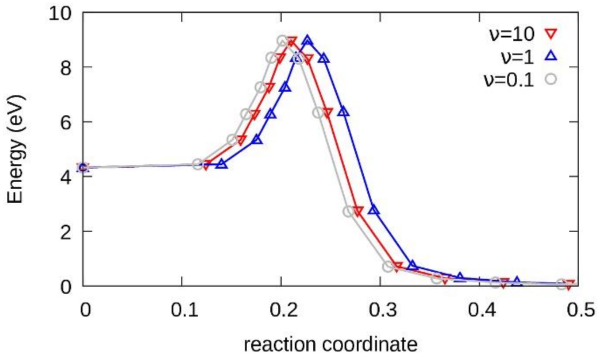


**Figure S13:** The potential energy along the MEP obtained using the modified NEB. Different curves correspond to different values of the parameter $\nu$, as indicated in the legend (units are $fs^{-1}$). The saddle point identified is independent of the value of $\nu$. The results were obtained using $N = 20$ images and only the region around the saddle point is shown.

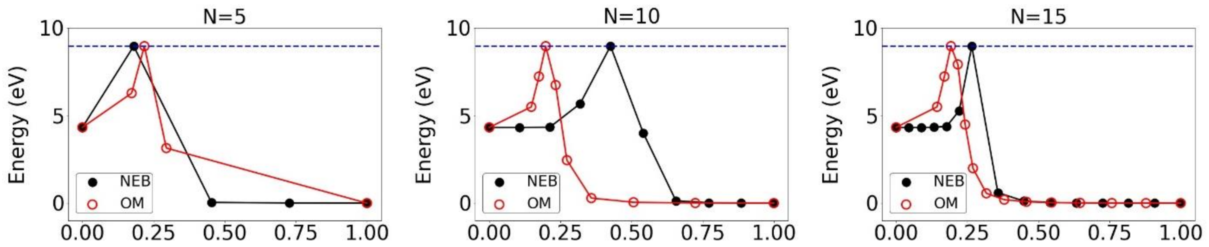


**Figure S14:** The potential energy along the MEPs obtained using an increasing number $N$ of images, as indicated in the title of each panel. The black and the red curves correspond to the results obtained using the standard and the modified NEB, respectively. The results reported here were obtained using $k_{\parallel} = 1$ eV/Å$^2$, $k_{\perp} = 0$ and $\nu = 1$ $fs^{-1}$. In each panel, the blue dashed line indicates the saddle point energy along the MEP. Both algorithms converge to the exact saddle point, independent of the number of images.

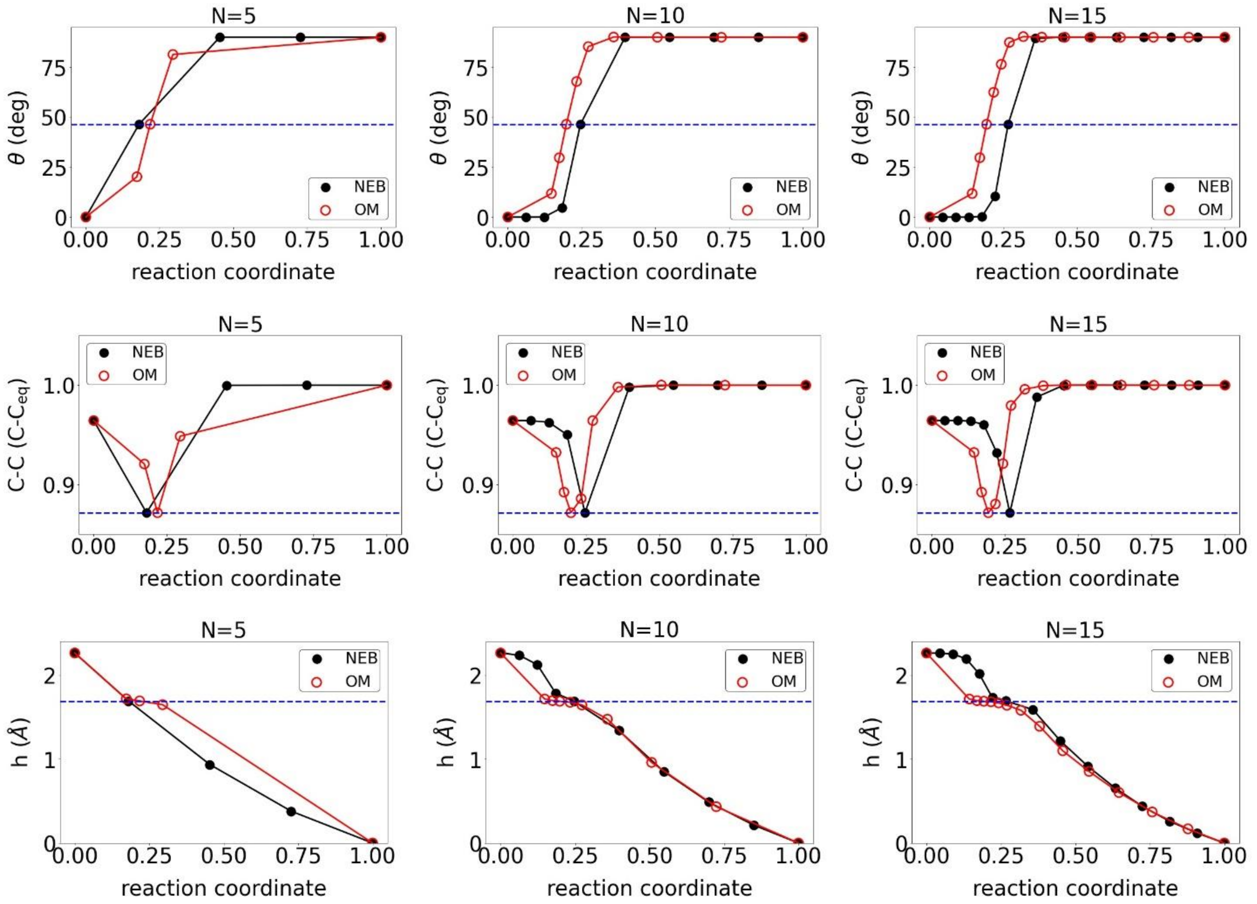


**Figure S15:** The angular orientation ($\theta$, first row) and the carbon-carbon bond length (C-C, second row) of the bond that undergoes the ninety degrees rotation, and the buckling amplitude of the graphene sheet ($h$, third row), plotted as a function of the reaction coordinate along the MEPs obtained using $N = 5, 10$ and 15 images, as indicated in the title of each panel. The black and the red curves correspond to the results obtained using the standard and the modified NEB, respectively. The results reported here were obtained using $k_{\parallel} = 1$ eV/Å$^2$, $k_{\perp} = 0$ and $\nu = 1$ fs$^{-1}$. The blue dashed line indicates the values at the saddle point.
